# Supplementary material for: Emergence and Dynamical Stability of Charge Time-Crystal in a Current-Carrying Quantum Dot Simulator
Source: arXiv:2205.06441 ancillary file (2022-05-13)
Supplement: Supplementary file 1 [file SI_for_pdl_Sarkar.pdf]

# Supporting Information: Emergence and Dynamical Stability of Charge Time-Crystal in a Current-Carrying Quantum-Dot Simulator

Subhajit Sarkar[∗,†] and Yonatan Dubi[∗,¶]

†*Department of Chemistry, Ben-Gurion University of the Negev, Beer Sheva 84105, Israel,*
‡*School of Electrical and Computer Engineering, Ben-Gurion University of the Negev, Beer Sheva 84105, Israel.*
¶*Department of Chemistry, Ben-Gurion University of the Negev, Beer Sheva 84105, Israel,*
§*Ilse Katz Center for Nanoscale Science and Technology, Ben-Gurion University of the Negev, Beer Sheva 84105, Israel.*

E-mail: subhajit@post.bgu.ac.il; jdubi@bgu.ac.il

## S1 Charge-FDS of the system

The total tunneling operator from chain $a$ to chain $b$ is identified with $\tau^+ = \sum_{k=1}^{N} \tau_k^+ = \sum_{k=1}^{N} c_{k,b}^{\dagger} c_{k,a}$. This is a dynamical symmetry operator for the system considered here as we

show explicitly. For the onsite terms corresponding to $\mathcal{H}_0$,

$$
\begin{aligned}
\sum_{j=1}^{N}\sum_{\alpha=a,b}\left[\epsilon_\alpha n_{j,\alpha},\tau_k^+\right] &= \sum_{j=1}^{N}\sum_{\alpha=a,b}\left[\epsilon_\alpha n_{j,\alpha}, c_{k,b}^\dagger c_{k,a}\right] \\
&= \sum_{j=1}^{N}\sum_{\alpha=a,b}\epsilon_\alpha\left(\left[n_{j,\alpha}, c_{k,b}^\dagger\right]c_{k,a} + c_{k,b}^\dagger\left[n_{j,\alpha}, c_{k,a}\right]\right) \\
&= \sum_{j=1}^{N}\sum_{\alpha=a,b}\epsilon_\alpha\left(\delta_{j,k}\delta_{\alpha,b} - \delta_{j,k}\delta_{\alpha,a}\right)c_{k,b}^\dagger c_{k,a} \\
&= (\epsilon_b - \epsilon_a)\tau_k^+, \qquad \text{(S1)}
\end{aligned}
$$

which implies the onsite term of the Hamiltonian the total tunneling operator $\tau^+$ is an eigen-operator with eigenvalue equal to the difference between the onsite energies of the ladder, viz., $(\epsilon_b - \epsilon_a)$. Furthermore, $\tau^+$ also commutes with the nearest-neighbor hopping part of the Hamiltonian,

$$
\begin{aligned}
&\left[-t_{||}^{hop}\sum_{j=1}^{N-1}\sum_{\alpha=a,b}\left(c_{j,\alpha}^\dagger c_{j+1,\alpha} + c_{j+1,\alpha}^\dagger c_{,\alpha}\right), \tau_k^+\right] \\
&= -t_{||}^{hop}\sum_{j=1}^{N-1}\sum_{\alpha=a,b}\left(c_{j,\alpha}^\dagger \delta_{k,j+1}\delta_{\alpha,b}c_{k,a} - c_{k,b}^\dagger\delta_{k,j}\delta_{\alpha,b}c_{j+1,\alpha}\right) \\
&= -t_{||}^{hop}\left(\sum_{k=2}^{N}c_{k-1,b}^\dagger c_{k,a} - \sum_{k=1}^{N-1}c_{k,b}^\dagger c_{k+1,a}\right) = 0. \qquad \text{(S2)}
\end{aligned}
$$

Moreover, it is easy to show that,

$$
\begin{aligned}
&\left[\left(\sum_{j=1}^{N}\sum_{\alpha=a,b}\frac{U}{2}n_{j,\alpha}n_{j,\alpha} + \sum_{j=1}^{N}U' n_{j,a}n_{j,b}\right), \tau_k^+\right] \\
&= (U-U')\tau_k^+(n_{k,b} - n_{k,a}) + (U-U')\tau_k^+, \\
&= 0, \text{ if } U = U',
\end{aligned}
$$

$$
\begin{aligned}
&\left[\sum_{j=1}^{N-1}\left(\sum_{\alpha=a,b}\frac{K}{2}n_{j,\alpha}n_{j+1,\alpha}+\frac{K'}{2}(n_{j,a}n_{j+1,b}+n_{j+1,a}n_{j,b})\right),\tau_k^+\right]\\
&= (K-K')\tau_k^+\Big(\frac{n_{k+1,b}+n_{k-1,b}}{2}+\frac{n_{k+1,a}-n_{k-1,a}}{2}\Big)\\
&= 0,\ \text{if } K=K'. \qquad \text{(S3)}
\end{aligned}
$$

Therefore, $[(\mathcal{H}_0+\mathcal{H}_{int}),\tau_k^+]=(\epsilon_b-\epsilon_a)\tau_k^+$, if $U=U'$ and $K=K'$. Considering the equal-time commutation relation the equation of motion for the total particle tunneling operator from chain $a$ to chain $b$, $\tau^+=\sum_{j=1}^N\tau_j^+$ become,

$$
\frac{d\tau^+}{dt}=i[H(t),\tau^+]+\frac{1}{2}\sum_\mu\left(V_\mu^\dagger\left[\tau^+,V_\mu\right]+\left[V_\mu^\dagger,\tau^+\right]V_\mu\right). \qquad \text{(S4)}
$$

We define total particle imbalance between the two chains of the ladder as $\tau_z=(N_b-N_a)/2=\sum_{j=1}^N\tau_j^z$ where $\tau_j^z=(n_{j,b}-n_{j,a})/2$ represents particle imbalance on each dimer $(j,a)-(j,b)$, and $\tau_j^x=\frac{\tau_j^++\tau_j^-}{2}$ and $\tau_j^y=\frac{\tau_j^+-\tau_j^-}{2i}$. Then the following commutation relations hold,

$$
\begin{aligned}
\left[\tau_j^\alpha,\tau_k^\beta\right] &= i\epsilon_{\alpha\beta\gamma}\tau_j^\gamma\delta_{jk},\ \alpha,\beta,\gamma=(x,y,z),\\
\left[(\mathcal{H}_0+\mathcal{H}_{hop}^{||}+\mathcal{H}_{int}),(N_b-N_a)/2\right] &= 0,\\
\left[(\mathcal{H}_0+\mathcal{H}_{hop}^{||}+\mathcal{H}_{int}),\tau^+\right] &= (\epsilon_b-\epsilon_a)\tau^+, \qquad \text{(S5)}
\end{aligned}
$$

where above equations signify that,

(i) the total particle imbalance $(N_b-N_a)$ between the two chains of the ladder is a conserved quantity, and

(ii) the total particle tunneling operator from chain $a$ to chain $b$ is a dynamical symmetry[1–3] in absence of driving,

indicating a hidden SU(2) symmetry due to the ladder structure. Moreover, for the lead

operators $V_{in} = \sqrt{\gamma_L} c^\dagger_{1,b}$ and $V_{out} = \sqrt{\gamma_R} c_{N,a}$ we find the following,

$$\begin{aligned} & V^\dagger_{in}[\tau^+_k, V_{in}] + [V^\dagger_{in}, \tau^+_k]V_{in} + V^\dagger_{out}[\tau^+_k, V_{out}] + [V^\dagger_{out}, \tau^+_k]V_{out} \\ = & -(\frac{\gamma_L}{2} c^\dagger_{1,b} c_{k,a} \delta_{k,1} + \frac{\gamma_R}{2} c^\dagger_{k,b} c_{N,a} \delta_{k,N}) \\ = & -\frac{\gamma_L}{2}\tau^+_1 - \frac{\gamma_R}{2}\tau^+_N. \end{aligned} \tag{S6}$$

Dephasing operator $V_{d,j} = \sqrt{\Gamma}(n_{j,a} + n_{j,b})$ also satisfy, $[V_{d,j}, \tau^+_k] = 0$ for arbitrary $j$ and $k$, indicating $\tau^+_k$ is a dark state operator with respect to the dephasing. Given the above commutation relations it is easy to show,

$$\sum_{j=1}^{N} \frac{d\tau^+_j}{dt} = \sum_{j=1}^{N} i[\mathcal{H}(t), \tau^+_j] - \frac{\gamma_L}{2}\tau^+_1 - \frac{\gamma_R}{2}\tau^+_N. \tag{S7}$$

Next we define a Floquet micro-motion operator,[4,5] $P(t) = e^{i\frac{\omega t}{2}(NI - \sum_j \tau^z_j)} = \prod_{\otimes j} e^{i\frac{\omega t}{2}(I - \tau^z_j)}$ with $P(t) = P(t+T)$ acting on the site basis, which will transform $\mathcal{H}(t)$ into the Floquet basis (rotated basis) where $H(t)$ is equivalent to a (stroboscopic) Floquet Hamiltonian under DC electric field $\mathbf{E} = (t^\perp_{hop}, 0, \Delta\epsilon - \omega)$, viz.,

$$\mathcal{H}_F = P(t)\left[\mathcal{H}(t) - i\partial_t\right]P^\dagger(t) = \mathcal{H}^{||}_{hop} + \mathcal{H}_{int} + \mathbf{E}\cdot\sum_j \boldsymbol{\tau}_j, \tag{S8}$$

where $\Delta\epsilon = \epsilon_b - \epsilon_b$ and $|\mathbf{E}| = \sqrt{(\Delta\epsilon - \omega)^2 + (t^\perp_{hop})^2}$. Equation (S8) signifies that in the spin-less model we have considered the charge-FDS is a consequence of an effective Stark Hamiltonian in the rotated frame, unlike the effective Zeeman Hamiltonian that appear in the spin-full system.[6,7] Therefore, from (S7) it is then easy to show,

$$\sum_j \frac{d\tau^+_{j,|\mathbf{E}|}}{dt} = \sum_j \left(i|\mathbf{E}| - \frac{\gamma_L}{2}\delta_{j,1} - \frac{\gamma_R}{2}\delta_{j,N}\right)\tau^+_{j,|\mathbf{E}|}, \tag{S9}$$

where the summation is over site index $j$ and we have assumed the effective field $\mathbf{E}$ is the same for each site (i.e., homogeneous) without the loss of the generality. Since the effective dipole

operators act locally on each dimer, this allows us to solve (S9) for each dimer separately

$$\begin{aligned}\tau^+_{1(N),|\mathbf{E}|}(T) &= \mathcal{U}_F\tau^+_{1(N),|\mathbf{E}|} = e^{i|\mathbf{E}|T}e^{-\frac{\gamma_{L(R)}T}{2}}\tau^+_{1(N),|\mathbf{E}|}\mathcal{U}_F \\ \tau^+_{j,|\mathbf{E}|}(T) &= \mathcal{U}_F\tau^+_{j,|\mathbf{E}|} = e^{i|\mathbf{E}|T}\tau^+_{j,|\mathbf{E}|}\mathcal{U}_F \;\forall\; j \neq 1 \text{ and } N,\end{aligned} \tag{S10}$$

which in absence of any charge transport through the system leads to a global charge-FDS, viz. $\mathcal{U}_F\tau^+_{|\mathbf{E}|} = e^{i|\mathbf{E}|T}\tau^+_{|\mathbf{E}|}\mathcal{U}_F$, and $[V_\mu, \tau^+_{|\mathbf{E}|}] = [V^\dagger_\mu, \tau^+_{|\mathbf{E}|}] = 0$. However, (S10) is not an exact relation at the operator level, rather it emerges near the FSS.[6]

Furthermore, it is easy to recognize that equation (S9) that equation of motion for $\tau^+_{|\mathbf{E}|}$ is generated by a Floquet Lindbladian $\mathcal{L}_F$ whose coherent part, $i\left[(\cdot), \sum_j \tau^+_{j,|\mathbf{E}|}\right]$, is generated by a Floquet Hamiltonian (S8). Therefore, from now on we work in the Floquet basis (in the rotated frame). We can define a local operator $\tau^+_{loc,|\mathbf{E}|} = \tau^+_{1,|\mathbf{E}|} + \tau^+_{N,|\mathbf{E}|} = (\underbrace{[\tau^+_{1,|\mathbf{E}|} \otimes I_2 \otimes \cdots \otimes I_N]}_{\text{block 1}} + \underbrace{[I_1 \otimes I_2 \otimes \cdots \otimes \tau^+_{N,|\mathbf{E}|}]}_{\text{block 2}})$. We then consider $\gamma_L = \gamma_R = \gamma$, i.e., the coupling between system with the left electrode is the same as that between the right electrodes, which is a standard assumption in transport setup. The local operator $\tau^+_{loc,|\mathbf{E}|}$ further satisfies $\mathcal{U}_F\tau^+_{loc,|\mathbf{E}|} = e^{i|\mathbf{E}|T}e^{-\gamma T/2}\tau^+_{loc,|\mathbf{E}|}\mathcal{U}_F$, and consequently after $l$ driving periods,

$$(\mathcal{U}_F)^l\tau^+_{loc,|\mathbf{E}|} = e^{il|\mathbf{E}|T}e^{-l\gamma T}\tau^+_{loc,|\mathbf{E}|}\mathcal{U}_F = e^{il|\mathbf{E}|T(1+i\gamma/2|\mathbf{E}|)}\tau^+_{loc,|\mathbf{E}|}. \tag{S11}$$

Defining Floquet coherence as

$$\rho_{mn} = (\tau^+_{loc,|\mathbf{E}|})^m\rho_{\text{FSS}}(\tau^-_{loc,|\mathbf{E}|})^n,\; m, n \text{ are positive integers,} \tag{S12}$$

for the Floquet steady state density matrix $\rho_{\rm FSS}$we arrive at weak charge-FDS,

$$\begin{aligned}
\mathcal{U}_F(\rho_{mn}) &= (\tau^+_{loc,|\mathbf{E}|})^m \mathcal{U}_F\left(\rho_{\rm FSS}(\tau^-_{loc,|\mathbf{E}|})^n\right) \\
&= e^{i(m-n)|\mathbf{E}|T} e^{-(m+n)\gamma T}(\tau^+_{loc,|\mathbf{E}|})^m \underbrace{[\mathcal{U}_F(\rho_{\rm FSS})]}_{\rho_{\rm FSS}}(\tau^-_{loc,|\mathbf{E}|})^n \\
&= e^{i(m-n)|\mathbf{E}|T} e^{-(m+n)\gamma T/2}\rho_{mn}, \qquad \text{(S13)}
\end{aligned}$$

that appears in Eq (5) of the main text.

## S1.1 Choice of dephasing operator

In deriving (S7) we have considered the dephasing operator of the form, $V_{d,j} = \sqrt{\Gamma}(n_{j,a} + n_{j,b})$ which satisfy, $[V_{d,j}, \tau^+_k] = 0$ because of the following relations: $[n_{j,a}, \tau^+_k] = -\tau^+_k \delta_{j,k}$, $[n_{j,b}, \tau^+_k] = \tau^+_k \delta_{j,k}$ implying $[(n_{j,a} + n_{j,b}), \tau^+_k] = 0$. If we were to choose an onsite dephasing such as $V_{d;j,a} = \sqrt{\Gamma} n_{j,a}$ and $V_{d;j,b} = n_{j,b}$ then the dissipator part of (S4) would give us,

$$\begin{aligned}
& V^\dagger_{d;j,a}[\tau^+_k, V_{d;j,a}] + [V^\dagger_{d;j,a}, \tau^+_k]V_{d;j,a} + V^\dagger_{d;j,b}[\tau^+_k, V_{d;j,b}] + [V^\dagger_{d;j,b}, \tau^+_k]V_{d;j,b} \\
= & \Gamma\left(n_{j,a}[\tau^+_k, n_{j,a}] + [n_{j,a}, \tau^+_k]n_{j,a} + n_{j,b}[\tau^+_k, n_{j,b}] + [n_{j,b}, \tau^+_k]n_{j,b}\right) \\
= & \Gamma\left([n_{j,a}, \tau^+_k] - [n_{j,b}, \tau^+_k]\right)\delta_{j,k} = -2\Gamma\tau^+_j\delta_{j,k}. \qquad \text{(S14)}
\end{aligned}$$

Therefore, with the on-site dephasing the dissipator part of (S4) corresponding to the dephasing operator does not vanish, leading complete elimination the DTC quantum coherence corresponding to $\tau^z_{|\mathbf{E}|}$ as mentioned in the main text.

The dephasing operator we choose here induces the charge-FDS. In QD array setup such a dephasing can in principle be induced via capacitive back-reaction from a nearby quantum-point contact (QPC) that simultaneously measure the charge in QDs at $(j, a) - (j, b)$ pair of cites.[8–11] The capacitive coupling between the QD and QPC appears due to the proximity effect[9,11] therefore, it is in principle possible to fabricate a device where the QPC has the same close proximity to both the QDs $(j, a) - (j, b)$ pair of cites thereby achieving the dephasing

necessary for charge-FDS.

## S2 Spectrum of Floquet propagator

For time periodic Liouvillian $\mathcal{L}(t+T) = \mathcal{L}(t)$ the time evolution super-operator (denoted by $\hat{\cdot}$) or the Floquet map is defined as,

$$\hat{\mathcal{U}}(t) = \mathcal{T}\left[\exp\left(\int_0^t \hat{\mathcal{L}}(t)\, dt'\right)\right], \tag{S15}$$

where $\mathcal{T}$ denotes the time time-ordering.[12] The one period time evolution operator is called the Floquet propagator and is defined as,

$$\hat{\mathcal{U}}_F = \mathcal{U}(T) = \mathcal{T}\left[\exp\left(\int_0^T \hat{\mathcal{L}}(t')\, dt'\right)\right], \tag{S16}$$

where the Liouvillian is given by the standard Markovian Floquet-Lindblad equation (2) of the main text.[5,13–15] Fig. S1 plots the spectrum of $\mathcal{U}_F$. The green squares correspond to the

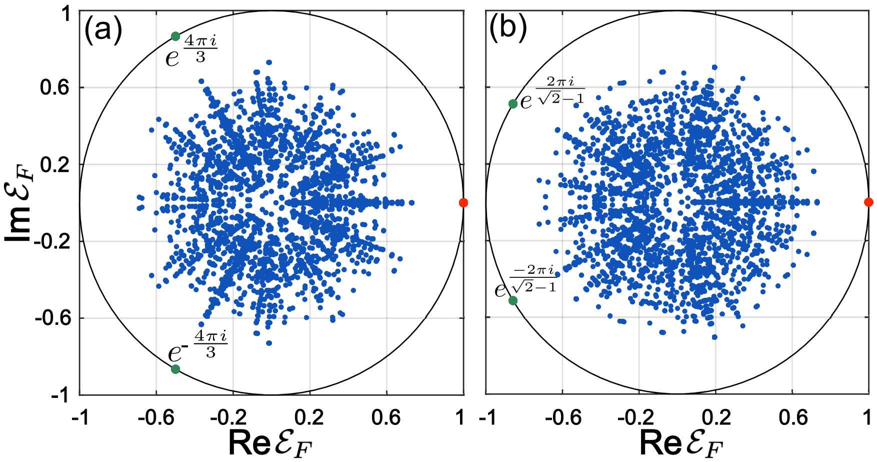


Figure S1: Plot of the spectrum of the Floquet propagator $\mathcal{U}_F|\rho\rangle\rangle = \mathcal{E}_F|\rho\rangle\rangle$, for N=3 which is the representative of a large system. The green squares on the peripheral (unit) circle represents the DTC state and the red square represents the Floquet steady states. Value of parameters: $t_{||}^{hop} = U = K = \omega = 20\pi MHz, (a) t_{\perp}^{hop} = \frac{4}{3}\omega$, and (b) $t_{\perp}^{hop} = \omega$ for $\gamma_L = \gamma_R = 10^{-4}\omega$.

eigen-value $e^{\frac{4\pi i}{3}}$ indicating the existence of a DTC in the system irrespective of any initial

condition.

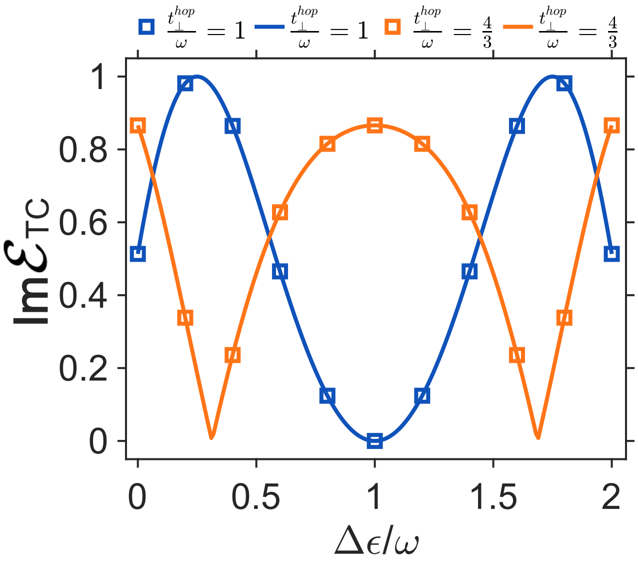


Figure S2: DTC/DTQC eigenvalues Im$[\mathcal{E}_{TC}]$ of $\mathcal{U}_F$ for various values of $\Delta\epsilon/\omega$, square data points are numerically obtained DTC /DTQC eigenvalues and solid lines correspond to Im $\left[e^{2\pi i(m-n)\frac{|\mathbf{E}|}{\omega}}\right] = \sin\left(2\pi r\frac{|\mathbf{E}|}{\omega}\right)$ obtained from weak-local charge-FDS, where $\gamma_L = \gamma_R = 10^{-4}\omega$. The system size considered for this plot is $N = 3$.

Fig. S2 plots the Imaginary part of the DTC eigenvalues $\mathcal{E}_F$ of $\mathcal{U}_F|\rho\rangle\rangle = \mathcal{E}_F|\rho\rangle\rangle$, viz., Im$[\mathcal{E}_{TC}]$ for small system-lead coupling $\gamma_L = \gamma_R = 10^{-4}\omega$, and shows that Im$[\mathcal{E}_{TC}]$ = Im $\left[e^{2\pi i(m-n)\frac{|\mathbf{E}|}{\omega}}\right]$ satisfying the weak-local charge-FDS condition (S11) after one period, i.e., $l = 1$. Fig. S2 signifies that by continuously changing $\Delta\epsilon$ one can reach a critical value $\Delta\epsilon_c$ for which Im$[\mathcal{E}_{TC}] = 0$, i.e., a purely real eigen-value of $\mathcal{U}_F$ with absolute value one, i.e., an eigenvalue corresponding to the red square in Fig. S1. A purely real eigenvalue of $\mathcal{U}_F$ further indicates that the system exhibits a Floquet response.

It is worthwhile to point out that the behavior gap in the spectrum of the Floquet map is a decisive factor for the stability of the DTC.[16] With the increase of the system size if the gap does not get closed then one can conclude the stability fo the DTC for a large system. However, numerically solving full spectrum of the Floquet map for the interacting many-body system we have considered is not only very challenging but also mostly out of reach of present day computational ability. That being said, the oscillation of the tunneling-

current, charge-current and the related frequency locking for system sizes ranging from N=2 to N=5 indirectly confirms that the said gap remain robust for larger system size for a specific system-lead coupling.

# S3 Decay of DTC due to system lead coupling

Here we show how the DTC oscillation decay when the system-lead coupling strength is increased. We take $t_{\perp}^{hop} = \frac{4}{3}\omega$, and $\omega$ for DTC and DTQC, respectively for $\gamma_L = \gamma_R = 10^{-2}\omega$. We investigate two cases, (i) when left and right electrodes attached to $(1, a)$ and $(N, b)$ sites, respectively, and (ii) when electrodes are attached to all the four boundary sites, i.e., left and right electrodes at $(1, a), (1, b)$ and $(N, a), (N, b)$, respectively.

Fig. S3 plots the DTC oscillation of $\langle \mathrm{Re}[\tau_j^+] \rangle$ for $\gamma_L = \gamma_R = 10^{-2}\omega$ showing the decay of the oscillation for a system with $N = 5$ for left and right electrodes attached to $(1, a)$ and $(N, b)$ sites, respectively. Fig. S3(a) shows that DTC oscillation decays very slowly at a time scale $2/\gamma$, Fig. S3(b) clearly showing $3T$ period of oscillation at the initial phase of the dynamics. In the long time limit Fig. S3(c) shows that the Floquet component have grown during the evolution signifying that the FSS component of the DTC density matrix has finite overlap with our chosen initial state. Fig. S3(d) shows the DFT of both oscillation of FDS operator and charge-current clearly showing the value $|\mathbf{E}|$ in the charge current.

Fig. S4 shows the DTC oscillation of $\langle \mathrm{Re}[\tau_j^+] \rangle$ for $\gamma_L = \gamma_R = 10^{-2}\omega$ when electrodes are attached to all the four boundary sites, i.e., left and right electrodes at $(1, a), (1, b)$ and $(N, a), (N, b)$, respectively, showing the decay of the oscillation for a system with $N = 5$. Fig. S3(a) shows that DTC oscillation decays very fast at a time scale $1/\gamma$. This can be understood from (S9), in this case (S9) will be replaced by the following,

$$\sum_j \frac{d\tau_{j,|\mathbf{E}|}^+}{dt} = \sum_j \left( i|\mathbf{E}| - \gamma_L \delta_{j,1} - \gamma_R \delta_{j,N} \right) \tau_{j,|\mathbf{E}|}^+, \tag{S17}$$

thereby making the decay twice as fast compared to the situation shown in Fig. S3. Fig.

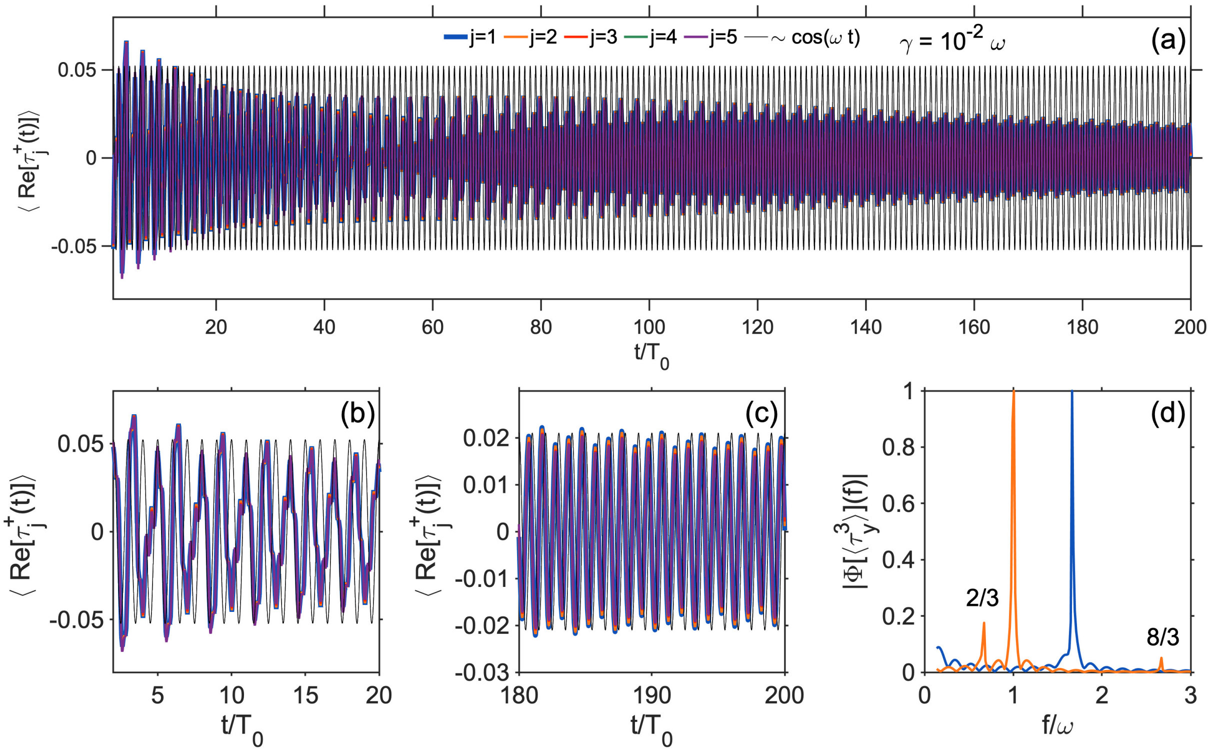


Figure S3: Plot of DTC oscillation for $\gamma_L = \gamma_R = 10^{-2}\omega$ showing the decay of the oscillation for a system with $N = 5$ for left and right electrodes attached to $(1, a)$ and $(N, b)$ sites, respectively. Plot of (a) $\langle Re[\tau_j^+](t)\rangle$ for long time duration up-to $200T$, (b) initial phase of the oscillation between $2T - 20T$, (c) oscillations in the long time limit between $180T - 200T$. (d) Discrete Fourier transform $|\tilde{\tau}_3^x(f)|$ of $\langle Re[\tau_j^+](t)\rangle$ and $|\tilde{J}_R(f)|$ of $\langle J_R(t)\rangle$ (oscillation not shown), respectively. The peak of $|\tilde{J}_R(f)|$ at 5/3 directly provides the value of the Floquet coherence. Value of parameters: $t_{||}^{hop} = U = K = \omega = 20\pi MHz,\ t_{\perp}^{hop} = \frac{4}{3}\omega$

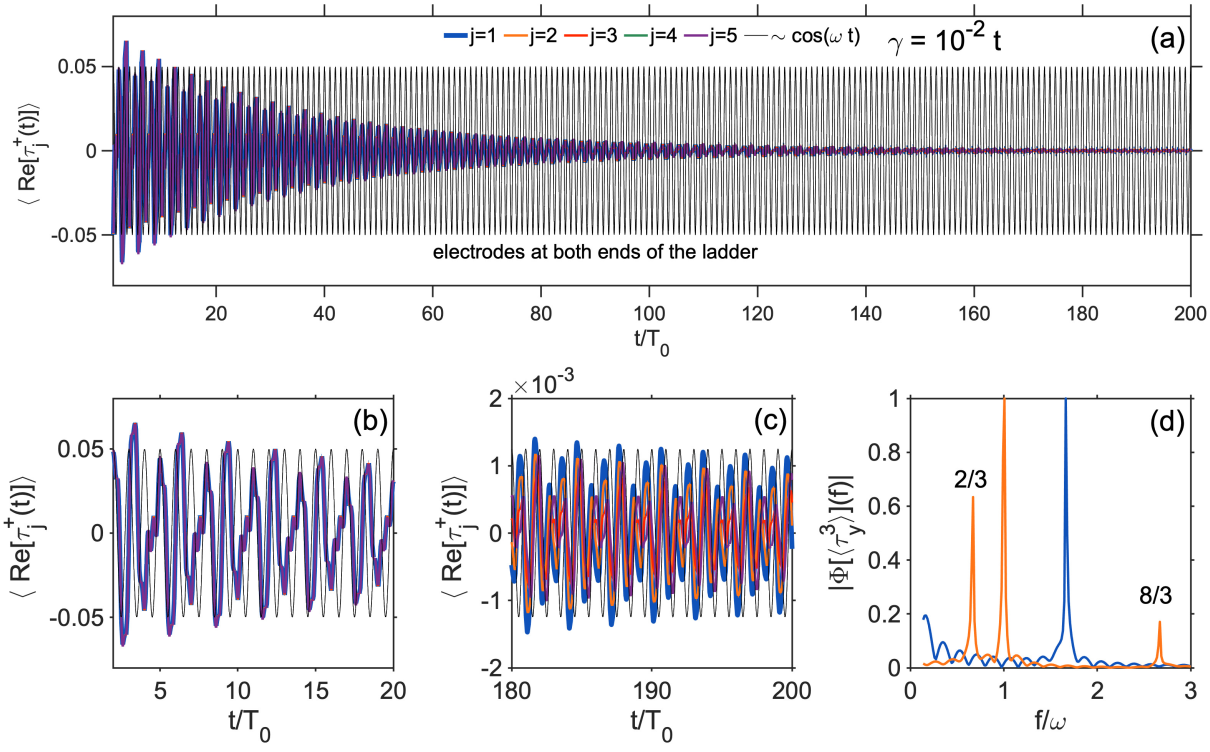


Figure S4: Plot of DTC oscillation for $\gamma_L = \gamma_R = 10^{-2}\omega$ showing the decay of the oscillation for a system with $N = 5$ and electrodes are attached to all the four boundary sites. Plot of (a) $\langle Re[\tau_j^+](t)\rangle$ for long time duration up-to $200T$, (b) initial phase of the oscillation between $2T - 20T$, (c) oscillations in the long time limit between $180T - 200T$. (d) Discrete Fourier transform $|\tilde{\tau}_3^x(f)|$ of $\langle Re[\tau_j^+](t)\rangle$ and $|\tilde{J}_R(f)|$ of $\langle J_R(t)\rangle$ (oscillation not shown), respectively. The peak of $|\tilde{J}_R(f)|$ at 5/3 directly provides the value of the Floquet coherence. Value of parameters: $t_{||}^{hop} = U = K = \omega = 20\pi MHz,\ t_{\perp}^{hop} = \frac{4}{3}\omega$

S4(b) clearly shows $3T$ period of oscillation at the initial phase of the dynamics. In the long time limit Fig. S4(c) shows that the Floquet component have not grown during the evolution signifying unlike the case of Fig. S3. This signifies that FSS component of the DTC density matrix obtained in this case has musch less finite overlap with our chosen initial state compared to the case of S3. Once again, Fig. S3(d) shows the DFT of both oscillation of FDS operator and charge-current clearly showing the value $|\mathbf{E}|$ in the charge current.

# S4 Current operator

In order to derive the charge-current operator we write the equation of motion of the number density at the site where the lead is connected, i.e., $n_{N\beta}$, where $\beta$ can be $a$ or $b$ or both depending on the position of the lead,

$$\begin{aligned}\frac{dn_{N,\beta}}{dt} &= i[\mathcal{H}(t), n_{N,\beta}] + \frac{1}{2}\sum_{\mu=\text{d, in, out}} \left(V_\mu^\dagger\left[n_{N,\beta}, V_\mu\right] + \left[V_\mu^\dagger, n_{N,\beta}\right]V_\mu\right), \\ &= it_{||}^{hop}\left(c_{N,\beta}^\dagger c_{N-1,\beta} - c_{N-1,\beta}^\dagger c_{N,\beta}\right) + it_\perp^{hop}\delta_{\beta,b}\left(c_{N,a}^\dagger c_{N,\beta}e^{i\omega t} - c_{N,\beta}^\dagger c_{N,a}e^{-i\omega t}\right) \\ &+ it_\perp^{hop}\delta_{\beta,a}\left(c_{N,b}^\dagger c_{N,\beta}e^{-i\omega t} - c_{N,\beta}^\dagger c_{N,b}e^{i\omega t}\right) - \gamma_R n_{N,\beta}, \\ &= (J_{hop} + J_{tunnel} - J_R)/e, \ e \text{ being the electronic charge} \end{aligned} \quad \text{(S18)}$$

where $[\mathcal{H}_{||}^{hop}, n_{N,\beta}] = it_{||}^{hop}\left(c_{N,\beta}^\dagger c_{N-1,\beta} - c_{N-1,\beta}^\dagger c_{N,\beta}\right)$, and $[\mathcal{H}_\perp^{hop}, n_{N,\beta}] = it_{hop}^\perp\delta_{\beta,b}\Big(c_{N,a}^\dagger c_{N,\beta}e^{i\omega t}$ $-c_{N,\beta}^\dagger c_{N,a}e^{-i\omega t}\Big) + it_\perp^{hop}\delta_{\beta,a}\left(c_{N,b}^\dagger c_{N,\beta}e^{-i\omega t} - c_{N,\beta}^\dagger c_{N,b}e^{i\omega t}\right)$, $[\mathcal{H}_{int}, n_{N,\beta}] = 0$ due to the fact that $\mathcal{H}_{int}$ depends only on the density of particles, and $\left(V_\mu^\dagger\left[n_{N,\beta}, V_\mu\right] + \left[V_\mu^\dagger, n_{N,\beta}\right]V_\mu\right) = 0$ for dephasing and left-lead. In (S18) hopping current from site $N-1,\beta$ to $N,\beta$ is given by $J_{hop}$, tunneling current from site $(j,a)$ to $(j,b)$ is given by $J_{tunnel}$ and the output current is given by, $J_{R,\beta} = e\gamma_R n_{N,\beta}$. The charge-current for the configuration of Fig. 1 is $J_R = e\gamma_R n_{N,b}$.

Charge current in the steady state is given by, $\langle J_R(t)\rangle = \mathrm{Tr}[J_R\rho_{DTC}(t)] = e\gamma_R\mathrm{Tr}[n_{N,b}\rho_{DTC}(t)]$ which are plotted in Fig. 2 and 4 in the main text.

# S5 Dynamical transition from DTQC to normal state

Here we show that the system can also make dynamical and reversible transition from a DTQC state to a state exhibiting Floquet response. We start form a value of $\Delta\epsilon = 0$ and then dynamically quench (by ramping) it to $\Delta\epsilon = 1$ for which $|\mathcal{E}| = \omega$. The quench profile is plotted in Fig. S5 Fig. S5 (b) and (c) plot $\langle \tau_j^x(t) \rangle$ and the charge current $\langle J_R(t) \rangle$ from

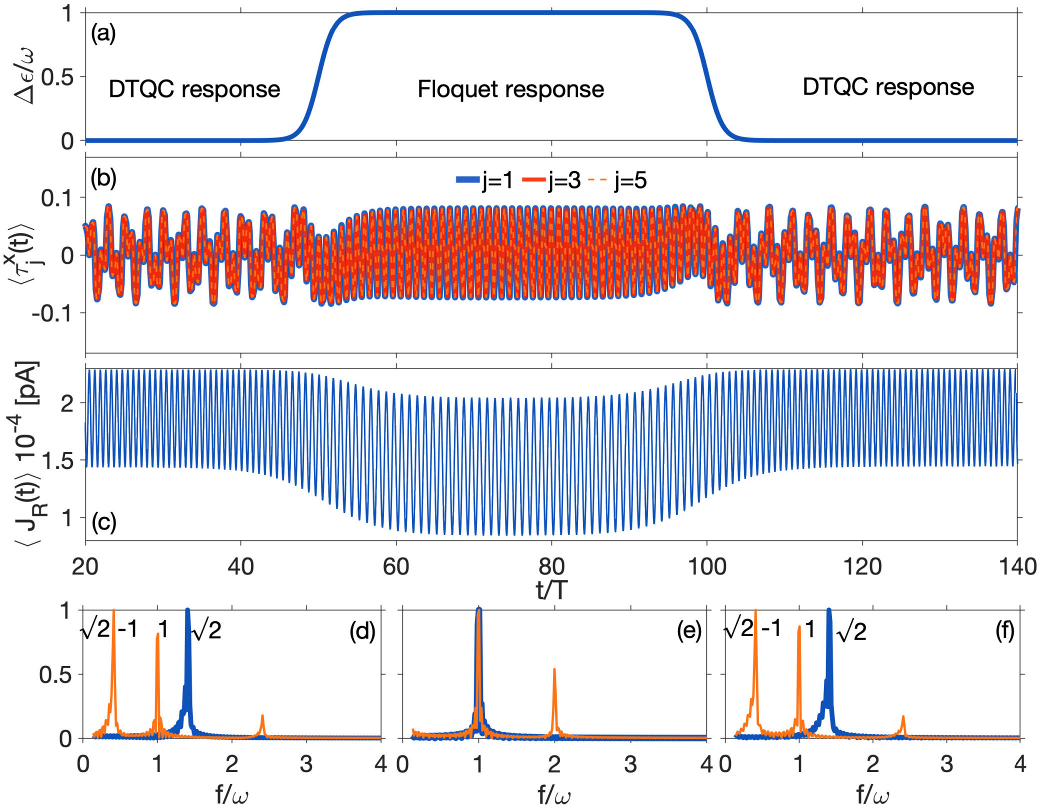


Figure S5: Dynamical cross-over between DTQC and normal phases. (a) Dynamical profile of the onsite energy $\epsilon_b/\omega$ as a function of time where $\epsilon_a/\omega = 0$. For a system with $N = 5$, (b) plot of $\langle \mathrm{Re}[\tau_j^+](t) \rangle$ , and (c) of charge current $\langle J_R(t) \rangle$, in $pA$ through right electrode as a function of time plotted over $140T$. (d), (e), and (f) Discrete Fourier transforms $|\tilde{\tau_3^x}(f)|$ of $\langle Re[\tau_j^+](t) \rangle$ and $|\tilde{J_R}(f)|$ of $\langle J_R(t) \rangle$, respectively between $5T - 45T$, $55T - 95T$, and $105T - 150T$, respectively. Value of parameters: $t_{||}^{hop} = t_{\perp}^{hop} = U = K = \omega = 20\pi\mathrm{MHz}$, $\gamma_L = \gamma_R = 10^{-4}\omega$, strong dephasing strength $\Gamma_d = \omega$ ensures fast synchronization.

the right lead, respectively, showing that the system dynamically enters, after a transient relaxation, into a normal state exhibiting Floquet response from a DTQC state once the system reaches the required critical value $\Delta\epsilon_c$, and again relaxes back to the DTC state

once the system is quenched away from $\Delta\epsilon_c$. Fig.S5 (d), (e), and (f) plot the DFTs of both $\langle \tau_j^x(t) \rangle$ and $\langle J_R(t) \rangle$ showing that the initial DTQC response exhibiting a peak at $\frac{|\mathbf{E}|}{\omega} = \sqrt{2}$ in the DFT of $\langle J_R(t) \rangle$, seen in Fig.S5 (d), is obtained back, as seen in Fig.S5 (f), after the system dynamically passes trough states exhibiting Floquet response with frequency $\omega$, seen in Fig.S5 (e).

## References


(1) Buča, B.; Tindall, J.; Jaksch, D. Non-stationary coherent quantum many-body dynamics through dissipation. *Nature Communications* **2019**, *10*, 1730.

(2) Tindall, J.; Muñoz, C. S.; Buča, B.; Jaksch, D. Quantum synchronisation enabled by dynamical symmetries and dissipation. *New Journal of Physics* **2020**, *22*, 013026.

(3) Medenjak, M.; Prosen, T.; Zadnik, L. Rigorous bounds on dynamical response functions and time-translation symmetry breaking. *SciPost Phys.* **2020**, *9*, 3.

(4) Shirley, J. H. Solution of the Schrödinger Equation with a Hamiltonian Periodic in Time. *Phys. Rev.* **1965**, *138*, B979–B987.

(5) Hartmann, M.; Poletti, D.; Ivanchenko, M.; Denisov, S.; Hänggi, P. Asymptotic Floquet states of open quantum systems: the role of interaction. *New Journal of Physics* **2017**, *19*, 083011.

(6) Sarkar, S.; Dubi, Y. Signatures of discrete time-crystallinity in transport through quantum dot arrays. *arXiv:2107.04214v2 [cond-mat.mes-hall]* **2021**, Fri, 9 Jul 2021.

(7) Chinzei, K.; Ikeda, T. N. Time Crystals Protected by Floquet Dynamical Symmetry in Hubbard Models. *Phys. Rev. Lett.* **2020**, *125*, 060601.

(8) Contreras-Pulido, L. D.; Bruderer, M.; Huelga, S. F.; Plenio, M. B. Dephasing-assisted transport in linear triple quantum dots. *New Journal of Physics* **2014**, *16*, 113061.

(9) Field, M.; Smith, C.; Pepper, M.; Ritchie, D.; Frost, J.; Jones, G.; Hasko, D. Measurements of Coulomb blockade with a noninvasive voltage probe. *Physical Review Letters* **1993**, *70*, 1311.

(10) Young, C.; Clerk, A. Inelastic backaction due to quantum point contact charge fluctuations. *Physical Review Letters* **2010**, *104*, 186803.

(11) Levinson, Y. Dephasing in a quantum dot due to coupling with a quantum point contact. *EPL (Europhysics Letters)* **1997**, *39*, 299.

(12) Riera-Campeny, A.; Moreno-Cardoner, M.; Sanpera, A. Time crystallinity in open quantum systems. *Quantum* **2020**, *4*, 270.

(13) Ho, T.-S.; Wang, K.; Chu, S.-I. Floquet-Liouville supermatrix approach: Time development of density-matrix operator and multiphoton resonance fluorescence spectra in intense laser fields. *Phys. Rev. A* **1986**, *33*, 1798–1816.

(14) Prosen, T.; Ilievski, E. Nonequilibrium Phase Transition in a Periodically Driven $XY$ Spin Chain. *Phys. Rev. Lett.* **2011**, *107*, 060403.

(15) Vorberg, D.; Wustmann, W.; Ketzmerick, R.; Eckardt, A. Generalized Bose-Einstein Condensation into Multiple States in Driven-Dissipative Systems. *Phys. Rev. Lett.* **2013**, *111*, 240405.

(16) Lieu, S.; Belyansky, R.; Young, J. T.; Lundgren, R.; Albert, V. V.; Gorshkov, A. V. Symmetry Breaking and Error Correction in Open Quantum Systems. *Phys. Rev. Lett.* **2020**, *125*, 240405.
